# Supplementary material for: Federated Foundation Models: Privacy-Preserving and Collaborative Learning for Large Models
Source: arXiv:2305.11414 source file (2024-03-19)
Supplement: Supplementary file 1 [file 09_appendix.tex]

\appendix
\section{Appendix}

\subsection{Background}
\subsubsection{Federated Learning}
% \subsubsection{Definition and characteristics}
Federated Learning~(FL) has been proposed as a distributed and privacy-preserving machine learning approach, which enables training on decentralized data without sharing private data between clients. FL shows extraordinary superiority on data privacy and security concerns, while facilitating collaborative learning across multiple clients. Key characteristics of federated learning include:
\begin{itemize}
\item Data is private and secure. Raw data remains on local clients, reducing the risk of data leaks and breaches.
\item Decentralized learning: Models are trained across multiple clients, leveraging the power of distributed computing.
\item Communication efficiency: Clients only share model updates (such as weights and gradients) asynchronously, not raw training data, reducing bandwidth requirements.
\end{itemize}

% \subsection{Federated learning architectures and algorithms}
% There are two primary federated learning architectures: horizontal and vertical federated learning.

% \begin{enumerate}
% \item \textbf{Horizontal Federated Learning:} Also known as sample-based federated learning, horizontal federated learning involves clients with the same feature space but different data samples. In this scenario, clients collaborate to train a global model using their local data, with the server aggregating and updating the global model. The most common algorithm used in horizontal federated learning is Federated Averaging (FedAvg) \cite{mcmahan2016communication}.
% \item \textbf{Vertical Federated Learning:} Also known as feature-based federated learning, vertical federated learning involves clients with different feature spaces but sharing the same data samples. In this scenario, clients collaborate on model training using secure multi-party computation techniques to ensure data privacy. The representative algorithm for vertical federated learning is SecureBoost \cite{cheng2019secureboost}.

% \end{enumerate}
% \subsubsection{Federated Averaging (FedAvg)}
Federated Averaging (FedAvg)~\cite{} is the most widely used algorithm for FL. 
It operates in several rounds, each consisting of a client-side local model training and a server-side global model aggregation. The FedAvg algorithm can be described as follows:

\begin{enumerate}
\item The server initializes the global model $w_0$ and sends it to all clients.
\item For each round $t = 1, 2, \ldots, T$:
\begin{enumerate}
\item The server selects a subset of clients $S_t$ to participate in the round.
\item Each client $k \in S_t$ receives the current global model $w_{t-1}$ and performs local model training by minimizing its local loss function $F_k(w)$ using stochastic gradient descent (SGD) or another optimization algorithm for $E$ epochs, yielding an updated local model $w_{t}^k$.
\item Each client $k \in S_t$ sends its local model update $\Delta w_t^k = w_t^k - w_{t-1}$ to the server.
\item The server aggregates the local model updates from clients and computes the new global model $w_t$ as follows:
\begin{equation}
w_t = w_{t-1} + \eta_t \sum_{k \in S_t} n_k \Delta w_t^k,
\end{equation}
where $\eta_t$ is the learning rate, and $n_k$ is the number of local data samples used by client $k$ for training.
\end{enumerate}
\end{enumerate}
% \subsection{Challenges and limitations}
Federated learning faces several challenges and limitations, including:

\begin{itemize}
\item {Non-IID data:} Data may be non-independent and identically distributed (non-IID) across clients, leading to difficulties in model convergence and performance.
\item {Communication overhead:} The exchange of model updates between clients and the central server can be time-consuming and resource-intensive, particularly for large models or when clients have limited bandwidth.
\item {Heterogeneous clients:} Clients may have varying computational resources, leading to discrepancies in local model updates and potential delays in global model convergence.
\item {Privacy and security:} While federated learning addresses many privacy concerns, it is still vulnerable to certain attacks, such as model inversion and membership inference attacks, requiring additional privacy-preserving techniques like differential privacy \cite{abadi2016deep}.
\end{itemize}
\subsection{Foundation Model Optimization}
% \section{Foundation Models: A Brief Overview}

\subsubsection{Definition and characteristics}
Foundation models are large-scale pre-trained machine learning models that serve as a starting point for downstream task-specific fine-tuning. These models, typically based on deep neural networks, capture a broad range of knowledge from diverse data sources and can be efficiently adapted to a wide array of tasks with minimal fine-tuning. Key characteristics of foundation models include:

\begin{itemize}
\item Pre-training: Foundation models are trained on massive datasets to learn general-purpose features and representations.
\item Transfer learning: These models can be fine-tuned with smaller labeled datasets for specific tasks, leading to improved performance and reduced training time.
\item Multi-modal and multi-task capabilities: Foundation models can be designed to handle various data modalities (e.g., text, images, audio) and multiple tasks simultaneously.
\end{itemize}

\subsection{State-of-the-art foundation models}
Several state-of-the-art foundation models have been developed in recent years, particularly in natural language processing (NLP) and computer vision (CV). Some notable examples include:

\begin{itemize}
\item \textbf{BERT} (Bidirectional Encoder Representations from Transformers) \cite{devlin2018bert}: A transformer-based model that has achieved groundbreaking results in various NLP tasks, including question answering, sentiment analysis, and named entity recognition.
\item \textbf{GPT} (Generative Pre-trained Transformer) \cite{radford2018improving}: Another transformer-based model initially designed for language modeling but has been successfully applied to a wide range of NLP tasks, with its latest version, GPT-3 \cite{brown2020language}, being one of the largest and most powerful language models available.

\item \textbf{ResNet} (Residual Networks) \cite{he2016deep}: A deep convolutional neural network (CNN) architecture for image recognition that introduced residual connections to alleviate the vanishing gradient problem, enabling the training of much deeper networks.

\item \textbf{ViT} (Vision Transformer) \cite{dosovitskiy2020image}: A transformer-based model adapted for computer vision tasks, such as image classification and object detection, which demonstrates the potential of transformers to generalize beyond NLP tasks.
\end{itemize}

\subsection{Challenges and limitations}
Despite their remarkable performance, foundation models face several challenges and limitations, including:

\begin{itemize}
\item \textbf{Computational resources:} Training foundation models requires substantial computational power and energy, which may not be accessible to all researchers and organizations.

\item \textbf{Data biases:} Foundation models can inherit biases present in their training data, which may lead to unintended consequences and ethical concerns when applied to real-world tasks \cite{bender2021dangers}.

\item \textbf{Model interpretability:} Due to their complex nature, understanding the decision-making process of foundation models remains a challenge, limiting their applicability in safety-critical and regulated domains.

\item \textbf{Adaptation to new tasks and domains:} While foundation models exhibit strong transfer learning capabilities, their performance may still be suboptimal for tasks or domains with limited available data or unique characteristics that deviate significantly from their pre-training data.
\end{itemize}

\subsection{Foundation Model Optimization}
% \section{Foundation Models: A Brief Overview}
% \subsubsection{Definition and characteristics}
Foundation Models~(FMs) are large-scale pre-trained machine learning models that serve as a starting point for downstream task-specific fine-tuning. These models, typically based on deep neural networks, capture a broad range of knowledge from diverse data sources and can be efficiently adapted to a wide array of tasks with minimal fine-tuning. Key characteristics of foundation models include:

\begin{itemize}
\item Pre-training: Foundation models are trained on massive datasets to learn general-purpose features and representations.
\item Transfer learning: These models can be fine-tuned with smaller labeled datasets for specific tasks, leading to improved performance and reduced training time.
\item Multi-modal and multi-task capabilities: Foundation models can be designed to handle various data modalities (e.g., text, images, audio) and multiple tasks simultaneously.
\end{itemize}

\subsubsection{State-of-the-art foundation models}
Several state-of-the-art foundation models have been developed in recent years, particularly in natural language processing (NLP) and computer vision (CV). Some notable examples include:

\begin{itemize}
\item \textbf{BERT} (Bidirectional Encoder Representations from Transformers) \cite{devlin2018bert}: A transformer-based model that has achieved groundbreaking results in various NLP tasks, including question answering, sentiment analysis, and named entity recognition.
\item \textbf{GPT} (Generative Pre-trained Transformer) \cite{radford2018improving}: Another transformer-based model initially designed for language modeling but has been successfully applied to a wide range of NLP tasks, with its latest version, GPT-3 \cite{brown2020language}, being one of the largest and most powerful language models available.

% \item \textbf{ResNet} (Residual Networks) \cite{he2016deep}: A deep convolutional neural network (CNN) architecture for image recognition that introduced residual connections to alleviate the vanishing gradient problem, enabling the training of much deeper networks.

\item \textbf{ViT} (Vision Transformer) \cite{dosovitskiy2020image}: A transformer-based model adapted for computer vision tasks, such as image classification and object detection, which demonstrates the potential of transformers to generalize beyond NLP tasks.
\end{itemize}
\subsubsection{Pre-training}
Pre-training is the initial phase in the development of foundation models, where models are trained on large-scale datasets to learn general-purpose representations. This process involves unsupervised or self-supervised learning techniques, such as language modeling for natural language processing (NLP) tasks, or contrastive learning for computer vision tasks. Pre-training aims to:

\begin{itemize}
\item Capture diverse knowledge and semantic structures from large-scale data sources.
\item Learn transferable representations that can be efficiently adapted to downstream tasks.
\item Reduce the need for extensive labeled data for task-specific fine-tuning.
\end{itemize}

Recent advances in pre-training techniques have focused on improving efficiency, scalability, and transferability of foundation models \cite{liu2021gpt}. For example, methods like layer-wise learning rate adaptation \cite{you2020large} and model distillation \cite{hinton2015distilling} have been proposed to speed up the pre-training process and reduce computational requirements.

\subsubsection{Fine-tuning and Transfer Learning}
Once the foundation models are pre-trained, they can be fine-tuned on specific tasks using smaller labeled datasets. Fine-tuning involves updating the model's parameters through supervised learning to optimize performance on the target task. There are several approaches to fine-tuning, including instruction tuning and multi-task tuning:

\begin{enumerate}
\item \textbf{Instruction Tuning:} This approach involves training the model to understand and follow natural language instructions, allowing it to generalize across a range of tasks with minimal explicit supervision \cite{schick2021exploiting}. Instruction tuning typically requires modifying the model's input and output formats and adapting its loss function to the specific task.

\item \textbf{Multi-task Tuning:} In this approach, the foundation model is fine-tuned on multiple tasks simultaneously, which encourages the model to learn shared representations that generalize across tasks \cite{ruder2017overview}. Multi-task tuning can involve training the model on a combination of tasks with shared or separate task-specific layers, and may require designing novel training objectives and evaluation metrics to balance the trade-offs between tasks.
\end{enumerate}

\subsubsection{Prompting and Zero-shot Learning}
Prompting and zero-shot learning are techniques that leverage the generalization capabilities of foundation models without requiring task-specific fine-tuning. These methods enable the models to perform new tasks by:

\begin{itemize}
\item \textbf{Prompting:} Providing the model with a carefully designed input query or prompt, which guides the model to generate the desired output. This approach relies on the model's pre-trained knowledge and its ability to understand and respond to natural language instructions \cite{shin2020autoprompt}.
\item \textbf{Zero-shot Learning:} Training the model to recognize and classify novel instances or concepts without any prior exposure to labeled examples from those classes. Zero-shot learning often involves the use of auxiliary information, such as class descriptions or semantic embeddings, to bridge the gap between the pre-trained model and the target task \cite{soares2019matching}.

\end{itemize}

\subsubsection{Challenges and limitations}
Despite their remarkable performance, foundation models face several challenges and limitations, including:

\begin{itemize}
\item \textbf{Computational resources:} Training foundation models requires substantial computational power and energy, which may not be accessible to all researchers and organizations.

\item \textbf{Data biases:} Foundation models can inherit biases present in their training data, which may lead to unintended consequences and ethical concerns when applied to real-world tasks \cite{bender2021dangers}.

\item \textbf{Model interpretability:} Due to their complex nature, understanding the decision-making process of foundation models remains a challenge, limiting their applicability in safety-critical and regulated domains.

\item \textbf{Adaptation to new tasks and domains:} While foundation models exhibit strong transfer learning capabilities, their performance may still be suboptimal for tasks or domains with limited available data or unique characteristics that deviate significantly from their pre-training data.
\end{itemize}

% \section{Background: Foundation Model Optimization}

Foundation models have demonstrated remarkable performance across a wide range of tasks and domains. However, there is still room for improvement in terms of efficiency, generalization, and applicability. This section provides an overview of the key optimization strategies employed for foundation models, which include pre-training, fine-tuning, and prompting and zero-shot learning.
